# Supplementary material for: Second-Order Dynamics in Noisy RNNs Produce Exploration and Temporal Compression in Replay
Source: arXiv:2611.29888 source file (2026-11-23)
Supplement: Supplementary file 1 [file ou_trained.tex]

\clearpage
\section{Trained Ornstein-Uhlenbeck Networks}

In \Cref{fig:1d_mean_std}, we simulated a theoretical network that has perfectly follows the score function of its optimal activity $r_{ou}(t)$ given that its observations $s_{ou}(t)$ follow an Ornstein-Uhlenbeck process.
Here we compare against this theoretical network simple, 10-neuron RNNs trained to path-integrate $s_{ou}(t)$, and see how replay from these networks might vary with nonlinearities (\Cref{fig:ou_vs_nonlinearity}) or with the presence of second-order modifiers in training (\Cref{fig:ou_vs_2nd_order_training}).
In \Cref{fig:ou_vs_nonlinearity}, we see the same trends from \Cref{fig:1d_mean_std} replicated in trained RNNs across nonlinearities.
In \Cref{fig:ou_vs_2nd_order_training}, we see that, if we incorporate second-order modifiers in RNN dynamics during training, the RNN adapts accordingly, meaning that these second-order modifiers become necessary during inference just to generate typical replay distributions.
This is in contrast to our main results, where we introduce second-order modifiers only during inference, so as to bias the resulting replay distributions.

\begin{figure}[h!]
\centering
\includegraphics[width=0.8\linewidth]{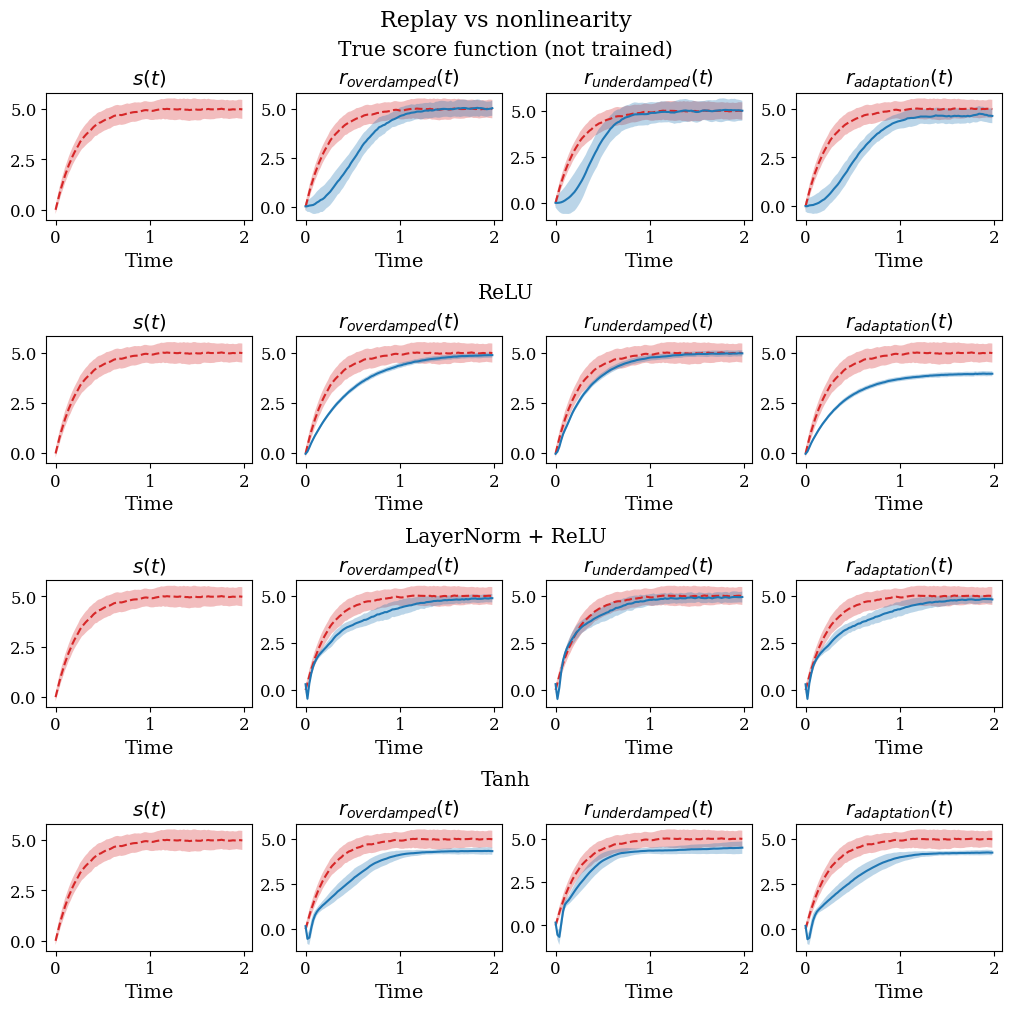}
\caption{Here we train three different 10-neuron RNNs (ReLU, LayerNorm + ReLU, and Tanh) on the Ornstein-Uhlenbeck path integration that the score-based dynamical system in \Cref{fig:1d_mean_std} is theoretically optimal for, and see how their replay distributions vary.
We see the same trends as in \Cref{fig:1d_mean_std} (top row).}
\label{fig:ou_vs_nonlinearity}
\end{figure}



\begin{figure}[h!]
\centering
\includegraphics[width=0.8\linewidth]{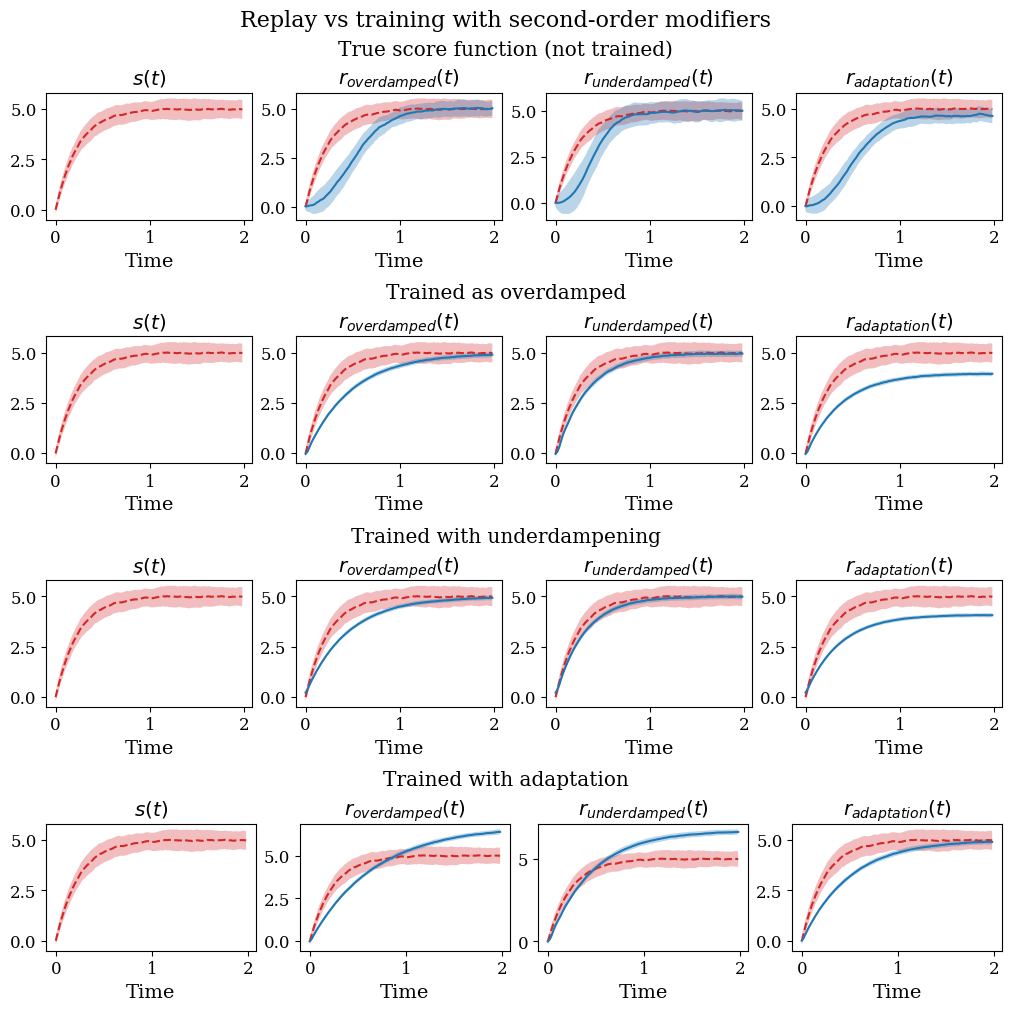}
\caption{Throughout all our results we incorporate second-order modifiers into RNN dynamics only during inference, never during training.
Here we investigate how replay might change if we incorporate these second-order modifiers during both trianing and inference.
We train a 10-neuron ReLU RNN on the same Ornstein-Uhlenbeck path integration task that the dynamical system from \Cref{fig:1d_mean_std} should be optimal for (top), except now we incorporate either none (overdamped), momentum (underdampening), or negative feedback (adaptation) into the RNN dynamics at both training and inference time.
We see that doing so makes these second-order modifiers mandatory during inference, thus weakening their ability to bias replay distributions compared to when we do not include them during training.
}
\label{fig:ou_vs_2nd_order_training}
\end{figure}
