# Supplementary material for: Second-Order Dynamics in Noisy RNNs Produce Exploration and Temporal Compression in Replay
Source: arXiv:2611.29888 source file (2026-11-23)
Supplement: Supplementary file 2 [file sufficient_conditions.tex]

\section{Sufficient Conditions for Offline Reactivation in RNNs}
\label{sec:appendix_sufficient_conditions}

The following proof is from \citet{sufficient_conditions}, who find an upper bound on the following loss $\loss \equiv \En{\bst - \bD\brt}$.
The key steps and assumptions they use to do so in the following equations are:
\begin{enumerate}
    \item Taylor expand $\mathcal{L}(t + \dt)$ around $t$ and keep only the linear terms.
    \item Assume that, after sufficiently successful training to minimize $\loss$, $p(\brt | \bst) \sim \mathcal{N}(\bDdag \bst, \sigmadt)$.
    \item Assume that $\bst \approx \bD\bDdag \bst$.
\end{enumerate}
%
\begin{align}
    \mathcal{L}&(t + \dt) =
    \En{\bs(t + \dt) - \bD(\brt + \drt{})} 
    \\
    &\approx
    \En{\bst + \bs'(t)\dt - \bD( \brt + \drt{})} \quad \text{(Taylor expansion around $t$)}
    \\
    &= \En{ \bs'(t) \dt - \bD \drt{2} + \bst - \bD( \brt + \drt{1} + \sigmaeta ) }
    \\
    &\leq \En{ \bs'(t) \dt - \bD \drt{2}} + \En{\bst - \bD( \brt + \drt{1} + \sigmaeta )}
    \\
    &= \norm{ \bs'(t) \dt - \bD \drt{2}} + \En{\bst - \bD( \brt + \drt{1} + \sigmaeta )}
    \\
    &\approx \norm{ \bs'(t) \dt - \bD \drt{2}} + \En{\bst - \bD( \bDdag \bst + \drt{1} + \sigmaeta )}
    \\
    &\approx \norm{ \bs'(t) \dt - \bD \drt{2}} + \En{\bD(\drt{1} + \sigmaeta )}
    \\
    &\leq \norm{ \bs'(t) \dt - \bD \drt{2}} + \lVert \bD \rVert_F \En{\drt{1} + \sigmaeta}
    \\
    &\leq \norm{ \bs'(t) \dt - \bD \drt{2}} + \lVert \bD \rVert_F \sqrt{\En{\drt{1} + \sigmaeta}^2}
    \quad \text{(Jensen's ineq.)}
    \\
    &\equiv \Lsignal(\drt{2}) + \Lnoise(\drt{1})
\end{align}


$\Lnoise$ minimizes $\En{\drt{1} + \sigmaeta}$, but could also be thought of as minimizing the variation of (i.e., denoising) $\br_{noisy}(t) \equiv \brt + \sigmaeta$ by adding $\drt{1}$. 
The optimal value for $\drt{1}$ is thus:
%
\begin{equation}
    \Delta \br_1^*(t) =
    \sigmadt~ \score,
\end{equation}
%
as proved in Section 2 of \citet{least_squares_estimation}, letting $y \leftarrow \br_{noisy}(t)$ and $x \leftarrow \brt$. 
Note that $\Delta \br_1^*(t)$ is simply the \textit{score function} of $\brt$ at time $t$, scaled by $\sigmadt$.
For multivariate Gaussian distributions, the score function has been derived in Appendix \ref{sec:appendix_score}.


The optimal RNN update equation can be obtained from Equations \ref{eq:rnn_update_definition} and \ref{eq:delta_r_1_and_2_star}:
%
\begin{equation} \label{eq:delta_r_star}
    \Delta \br^*(t + \dt) =
    \left[
    \sigma_r^2 \score)
    +
    \bDdag \bs'(t)
    \right] \dt + \sigmaeta
\end{equation}
