# Supplementary material for: Second-Order Dynamics in Noisy RNNs Produce Exploration and Temporal Compression in Replay
Source: arXiv:2611.29888 source file (2026-11-23)
Supplement: Supplementary file 3 [file temp.tex]

\section{Introduction}

\paragraph{What is replay?}
Neural circuits undergo active, input-driven periods and quiescent, undirected periods (like sleep or wakeful rest).
During the latter, some circuits can internally generate activity resembling the former \citep{tingley2020methods}.
Such phenomena have been observed in the prefontal \citep{euston2007fast, peyrache2009replay}, sensory \citep{kenet2003spontaneously, xu2012activity}, motor \citep{hoffman2002coordinated}, and entorhinal cortices \citep{gardner2022toroidal}; the anterior thalamus \citep{peyrache2015internally}; head direction systems \citep{peyrache2015internally}; and the hippocampus \citep{sleep_loss, content_of_hippocampal, replay_of_neuronal, igata2021prioritized, hippocampal_replay_is_not, hippocampal_reactivation_random, hippocampal_sharp_wave_ripple, hippocampal_sharp_waves, integration_and_segregation, superficial_layers, nadasdy1999replay, lee2002memory, foster2017replay, memory_and_brain, offline_ensemble}.
Of those circuits, the hippocampus is particularly interesting because its robustness in tasks like navigation \citep{hippocampus_cognitive_map, model_hippocampal, deciphering_hippocampal, memory_navigation_theta}, memory \citep{loss_recent_memory, prefrontal-hippocampal, place_navigation_impaired, optogenetic_stimulation}, planning \citep{hippocampal_place-cell_sequences, dorsal_hippocampus, hippocampal_theta_sequences_reflect}, and imagination \citep{role_hippocampus_prediction, patients_hippocampal_amnesia} during active, awake states seems crucially tied to its spontaneous activity during quiescent or sleep states \citep{two-stage_model, hippocampal_sharp_wave_ripple, sleep_price}.


\paragraph{Why is replay useful?}
Indeed, many characterizations of spontaneous activity during quiescence focus on the hippocampus because of a clear duality in hippocampal operation: during wakefulness, hippocampal activity tracks environment or task variables (like position) \citep{learning_produces_hippocampal, geometric_transformation, latent_learning, from_cell_types}, while during rest, spontaneous hippocampal activity resembles a ``replay'' of wakeful activity that may serve a myriad of functions \citep{content_of_hippocampal, replay_of_neuronal, igata2021prioritized, hippocampal_replay_is_not, hippocampal_reactivation_random, hippocampal_sharp_wave_ripple, hippocampal_sharp_waves, integration_and_segregation, superficial_layers, nadasdy1999replay, lee2002memory, foster2017replay, memory_and_brain, evolving_view}.
%
Functions of neural replay may include memory consolidation and maintenance \citep{buzsaki1989two, mcclelland1995there, awake_replay_off, paradoxical_replay, large_sharp_wave, hippocampal_replay_awake, role_hippocampal_replay, parallel_processing, local_inhibitory_circuits, lewis2011overlapping, offline_ensemble, recurrent_network_model, replay_basis_backprop}, decision-making and planning of future actions \citep{olafsdottir2015hippocampal, igata2021prioritized, awake_replay_off, constant_sub-second, sampling_motion_trajectories, time_course_organization, internally_generated, preplay_future_place, reward_revaluation}, and sampling and uncertainty representation \citep{sampling_motion_trajectories, left_right_alternating, replay_compositional}.
%
Replay is also beneficial for artificial systems to circumvent training data scarcity \citep{mnih2015human} and prevent catastrophic forgetting \citep{hayes2019memory, memory_replay_data, compressed_latent_replays, brain_like_replay}, but designing performant neural networks that can both perform tasks and generate replay remains an open question \citep{sufficient_conditions, sequential_predictive_learning, brain_like_replay}.



\paragraph{How have people modeled replay before?}

While some works have tried to produce replay via supervised generative models \citep{deperrois2022learning}, in most existing models of hippocampal activity, replay is an emergent byproduct of careful network design.
Relevant network parameters include connectivity structures \citep{shen1996modeling, azizi2013computational, milstein2023offline}, local plasticity mechanisms \citep{hopfield2009neurodynamics, litwin2014formation, theodoni2018theta, haga2018recurrent, asabuki2023learning}, firing rate adaptation \citep{chu2023firing, computational_model_preplay, cell_assembly_sequences, nrem_sleep, noisy_adaptation, dynamics_of_adaptive_canns, sequential_predictive_learning}, and input modulation \citep{kang2019replay}.
Some of the most common hippocampal circuit models are continuous attractor neural networks (CANNs) \citep{path_integration, attractor_neural_networks_storing, attractor_neural_network_models, canns_candidates}, since they use spatially tuned cells \citep{hippocampus_cognitive_map} and produce stable, low-dimensional activity \citep{attractor_and_integrator, learning_produces_hippocampal, geometric_transformation, latent_learning}, even in the absence of directed input \citep{noisy_adaptation, continuous_attractors_dynamic,  stability_of_working_memory}.
However, CANNs and other traditional hippocampus models cannot account for the role of weakly tuned cells (which contribute to low-dimensional activity \citep{latent_learning, collective_behavior_place} and distributed representations of space \citep{manifold_neural_population, distributed_neural_code}) and, most importantly, do not describe how hippocampal representations and networks may be learned from data.




\paragraph{Sequential predictive learning.}

One promising model of hippocampal function with emergent replay is sequential predictive learning, wherein hippocampal circuits must track (i.e., predict) dynamic environment or task variables from imperfect observations thereof.
For example, predicting upcoming positions from a history of position-related measurements (like velocity); in other words, \textit{path-integrating} the position.
%
This normative description of hippocampal function as sequence prediction matches hippocampal encodings of upcoming stimuli \citep{hippocampus_preserves_order} and prediction errors \citep{hippocampal_representations_switch, emergence_predictive_model}, anatomical features of the hippocampus \citep{computational_approach, sequence_predicting_ca3, predictive_sequence_learning}, and observations of neural activtity sweeps that represent trajectories of possible future positions \citep{constant_sub-second, neural_ensembles_ca3, sampling_motion_trajectories}.
Unlike traditional, hand-crafted models, sequential predictive learning models are trained from data.
%
Nonetheless, they account for the emergence of spatially-tuned neurons \citep{predictive_learning_network_mechanism, automated_mapping, sequential_predictive_learning, predictive_sequence_learning}, grid cells \citep{cueva2018emergence, sorscher2019unified, excitatory_inhibitory_recurrent, conformal_isometry, learning_grid_cells}, and head direction cells \citep{Cueva2020Emergence, Uria2020Spatial}; link hippocampal function and reinforcement learning \citep{hippocampus_predictive_map, predictive_representations_link}; can incorporate phenomena like theta oscillations \citep{sequential_predictive_learning, generative_model_hippocampal}; and exhibit quiescent replay activity \citep{sufficient_conditions, sequential_predictive_learning, predictive_sequence_learning}.
%
Additionally, there exist connections between traditional CANN and trained RNN models of hippocampal function, since RNNs can approximate or be combined with continuous attractors \citep{emergence_robust, back_continuous, predictive_learning_energy, sequential_predictive_learning, sorscher2019unified}.
%
While previous work has analytically shown that sequential predictive learning networks act as generative models during quiescent activity \citep{sufficient_conditions}, to our knowledge no additional works have theoretically characterized the statistics of quiescent activity in trained networks.




\paragraph{Exploration and temporal compression in replay.}

Two particularly interesting and commonly reported phenomena in models of neural replay are \textit{exploration} and \textit{temporal compression}.
%
Exploration is notion that quiescent neural activity (i.e., replay) expresses a variety of behavioral sequences, whether they be reexpressions of awake activity or entirely novel syntheses \citep{evolving_view, hippocampal_place-cell_sequences, hippocampal_replay_is_not, hippocampal_reactivation_random, hippocampal_replay_extended}---in other words, replay \textit{explores} the space of possible neural trajectories. 
Phenomena associated with exploration in replay include long trajectories in neural space, visitation of multiple attractor basins, and transitions that were not present in awake activity.
One key method to induce exploration in models of replay is through negative feedback on activity, or \textit{neural adaptation}, which can destabilize attractors and induce sudden transitions in replay activity \citep{sequential_predictive_learning, noisy_adaptation, dynamics_of_adaptive_canns, cell_assembly_sequences}, and is thought to play a key role in the dynamics of replay \textit{in vivo} \citep{nrem_sleep}.
%
%
Another salient characteristic of replay is the timescale: replay sequences are often much faster (or even reversed \citep{reverse_replay_behavioural, evolving_view, recurrent_network_model}) compared to awake sequences of activity, exhibiting a temporal compression thereof \citep{emergence_preconfigured, nadasdy1999replay, speed_time_compressed, hippocampal_sharp_wave_ripple, memory_sequential_experience, evolving_view, fragmented_replay, hippocampal_replay_extended}.
%
This compression could be a byproduct of memory compression \citep{working_memory_capacity, nadasdy1999replay, fragmented_replay}, which is itself closely tied to phase precession, wherein neurons encode sequences through a temporal code that occurs progressively earlier relative to local theta oscillations \citep{phase_relationship, theta_phase_precession_hippocampal, position_reconstruction, theta_phase_precession_supports}.
%
While various mechanisms have been proposed to underlie phase precession \citep{theta_phase_precession_beyond, phase_precession_neural_code}, of particular relevance to our work are reports of short-term facilitation (which could be implemented in hippocampal mossy fiber synapses), combined with membrane potential oscillations, inducing phase precession \citep{temporal_compression_mediated, phase_precession_through}.
%
While observations of exploration and temporal compression in replay are abundant, models thereof are scarce, especially in trained RNNs: only recently has exploration been observed in replay from trained RNNs \citep{sequential_predictive_learning},  and to date there are no models of temporal compression in replay from trained RNNs.


\subsection{Contributions (problem + result)}

While sequential predictive learning is a promising new model of hippocampal function and replay, its empirical scope is quickly outpacing its theoretical foundations.
Theoretical work has established that path-integrating RNNs synthesize novel trajectories during quiescent activity through a variant of Langevin sampling \citep{sufficient_conditions}.
However, subsequent work has introduced new mechanisms to qualitatively bias quiescent activity without a rigorous description of said biases \citep{sequential_predictive_learning}.
\josue{Connect these biases to the phenomena from earlier}
Moreover, it is unclear whether additional mechanisms might exist to bias quiescent activity, incorporate other phenomena like temporal compression, or reveal universal patterns of RNN design for replay.
\josue{Be explicit about what experimental observations \citep{sufficient_conditions} and previous models cannot account for}

We remedy these shortcomings of sequential predictive learning for replay by characterizing how RNN design and Langevin sampling \josue{statistics} affect other.
%
Some of our results describe how recent RNN design mechanisms affect Langevin sampling statistics of replay, such as speed and variance.
Meanwhile, our other results start from the Langevin sampling formulation of replay and either explain existing architectural choices as useful inductive biases, or propose new RNN design mechanisms to again modulate sampling.
In summary, the three questions we answer are:

%While noisy RNNs are promising models of neural replay, little is known about them compared to traditional CANNs:
%
%\begin{enumerate}
%\item The relationships between input statistics, RNN parameters, and Langevin sampling are unclear.
%Current RNN Langevin sampling theories are limited by assumptions of stationary input statistics \citep{sufficient_conditions}, and cannot explain the role of even simple architectural parameters like hidden state leakage.
%\item Biologically inspired mechanisms of neural adaptation and masked training are useful for neural replay, but how they affect Langevin sampling and replay statistics is not fully clear.
%\item Modern generative (i.e., diffusion) models benefit from modified (annealed) Langevin dynamics \citep{generative_modeling_by_estimating_gradients}, but whether noisy RNNs could also benefit from novel sampling techniques is unknown.
%\end{enumerate}

%We use Langevin sampling theory to remedy the above shortcomings of neural replay in noisy RNNs by answering the following questions:
%
\begin{enumerate}
\item Langevin sampling requires estimating the score function of a distribution.
In RNNs, what is the nature of this function, and might it have intrinsic properties that inform architectural choices?
\textit{The score function is time-variant and thus difficult to estimate, even for simple distributions---however, our expression of it motivates the addition of linear dynamics (leakage) in RNNs.}
%
\item Negative feedback (adaptation) and multi-step (masked) training empirically induce exploration and coherence, respectively, in replay.
How do they affect Langevin sampling?
\textit{Adaptation induces non-Markov second-order Langevin sampling that destabilizes attractors, which can both help (diversify) and hurt (slow) replay; masked training forces the RNN to learn both its score function and the dynamics of observed events.}
%
\item Traditional generative models benefit from a wide array of sampling techniques. Could new sampling methods improve replay in noisy RNNs?
\textit{Underdamped Langevin sampling via momentum quickens neural replay, like temporal compression induced by short-term facilitation} in vivo\textit{, and mitigates slowing from adaptation while maintaining exploration.}
\end{enumerate}


















\section{Related Work}

\paragraph{Sequential predictive coding and path integration in RNNs.}

Our work adds to a growing literature of predictive coding in RNNs.
While predictive representations have long been theorized to be a fundamental component of neural computation or even plasticity \citep{neural_mechanisms_predictive, predictive_coding, predictive_coding_review, predictive_coding_dynamical, relationship_predictive_coding_backprop}, one of the first observations of them in trained RNNs emerged as a byproduct of energy constraints (activation penalties) \citep{predictive_coding_consequence}.
%
Whatever the origin of predictive representations may be, many other works have examined their properties in RNNs---specifically, the properties of representations learned from path integration, or prediction of future elements in sequences from nonlinear, noisy, or indirect observations of previous elements.
%
Indeed, several works have shown path integration inducing salient hippocampal properties like sequential memories \citep{sequential_memory} (similar to memories in energy-based Hopfield networks \citep{neural_networks_physical}) and place or grid cell representations \citep{learning_grid_cells, sequential_predictive_learning, predictive_sequence_learning, sorscher2019unified, excitatory_inhibitory_recurrent, conformal_isometry}
%
Most crucial to our work are observations of replay as a consequence of path integration in RNNs \citep{sufficient_conditions, sequential_predictive_learning, predictive_sequence_learning}.




\paragraph{Data-driven RNN models of replay.}

Our work builds upon recent data-driven models of replay in RNNs\footnote{
These works and ours focus on diffusive replay \citep{hippocampal_reactivation_random} that is stationary insofar as the set of training sequences used to induce replay is fixed, as opposed to descriptions of \textit{in vivo} replay as non-stationary over coarse timescales like days \citep{cortical_reactivations_predict, time_course_organization}.
}.
%
\citet{sufficient_conditions} proved and empirically confirmed that path-integrating RNNs perform a variant of Langevin sampling during quiescent, undirected periods of activity.
This Langevin sampling description of activity is the foundation of our findings: we ask how this description might inform network design, and we use this description to understand how second-order activity modulators like adaptation (negative feedback) and momentum bias distributions of replay activity.
%
\citet{sequential_predictive_learning} show that sequential predictive coding RNNs resemble CANNs---with low dimensional, coherent representations and non-trivial replay trajectories---even in complex environments, and find new, biologically plausible, ways of training and modifying said RNNs to ensure CANN-like behavior.
We analytically examine these modifications of RNN activity and training (adaptation and masked training, respectively) through the lens of Langevin sampling, and introduce a new modifier in the form of momentum.
%
\citet{predictive_sequence_learning} map components of sequential predictive RNNs onto specific subregions of the hippocampus, and again confirms the occurrence of phenomena like replay.
Their findings do not directly influence our work, but are a useful reference for discussions of how the computational models we use could be implemented \textit{in vivo}.


\paragraph{RNNs and Langevin generative models.}
Throughout this work we treat RNNs as generative models using a variant of Langevin sampling.
Expressive generative models, in particular \textit{diffusion models} whose activity resembles Langevin sampling, have received much attention from the machine learning community \citep{self_consuming, boomerang, diffusion_models_comprehensive, diffusion_models_in_vision, diffusion-lm, chatgpt_is_not, generative_modeling_by_estimating_gradients}.
The fundamental differences between our RNNs and diffusion models are twofold.
The first is that each timestep of a generated replay trajectory is generated sequentially and with only one effective step along the gradient of log-likelihood, whereas a diffusion model would generate all timesteps of a path simultaneously and with many steps along the gradient of log-likelihood.
The second is that diffusion models use time-varying noise levels (annealed dynamics) and are explicitly conditioned on time as an input, whereas our RNNs use the same noise level across time and are never explicitly conditioned on time.
